# Supplementary material for: Path Similarity Analysis: a Method for Quantifying Macromolecular Pathways
Source: arXiv:1505.04807 ancillary file (2015-10-23)
Supplement: Supplementary file 1 [file S1_Table.pdf]

---

# Supporting Information

**S1 Tab.** Numerical values for domain angles for experimental crystal structures of AdK.

---

## References

- [1] Beckstein O, Denning EJ, Perilla JR, Woolf TB. Zipping and Unzipping of Adenylate Kinase: Atomistic Insights into the Ensemble of Open  $\leftrightarrow$  Closed Transitions. *J Mol Biol.* 2009 Nov;394(1):160–176.
- [2] Beckstein O, Denning EJ, Woolf TB. AKeco Structure Library; 2015. Available from: <http://dx.doi.org/10.5281/zenodo.29243>.

**Table 1. Domain angles for experimental crystal structures of AdK.**

| PDB ID | chain | NMP-CORE | LID-CORE |
|--------|-------|----------|----------|
| 1AK2   | A     | 71.6°    | 97.9°    |
| 1AKE   | A     | 45.3°    | 106.1°   |
|        | B     | 44.7°    | 106.7°   |
| 1AKY   | A     | 43.8°    | 112.1°   |
| 1ANK   | A     | 45.5°    | 107.3°   |
|        | B     | 45.2°    | 106.9°   |
| 1DVR   | A     | 67.4°    | 113.2°   |
|        | B     | 69.8°    | 108.9°   |
| 1E4V   | A     | 45.1°    | 105.8°   |
|        | B     | 45.0°    | 105.8°   |
| 1E4Y   | A     | 44.6°    | 111.5°   |
|        | B     | 45.1°    | 116.0°   |
| 1P3J   | A     | 44.1°    | 109.5°   |
| 1S3G   | A     | 45.9°    | 108.7°   |
| 1ZAK   | A     | 45.9°    | 120.3°   |
|        | B     | 45.9°    | 114.9°   |
| 1ZIN   | A     | 45.7°    | 122.9°   |
| 1ZIO   | A     | 45.1°    | 124.8°   |
| 1ZIP   | A     | 45.3°    | 123.5°   |
| 2AK2   | A     | 69.4°    | 101.3°   |
| 2AK3   | A     | 50.5°    | 154.4°   |
|        | B     | 53.4°    | 164.7°   |
| 2AKY   | A     | 43.1°    | 109.0°   |
| 2AR7   | A     | 63.2°    | 119.4°   |
|        | B     | 56.0°    | 131.0°   |
| 2BBW   | A     | 56.0°    | 128.1°   |
|        | B     | 57.0°    | 116.7°   |
| 2C9Y   | A     | 65.4°    | 89.2°    |
| 2ECK   | A     | 45.2°    | 106.3°   |
|        | B     | 45.1°    | 106.8°   |
| 2EU8   | A     | 44.3°    | 113.3°   |
|        | B     | 44.1°    | 111.6°   |
| 2O07   | A     | 44.2°    | 112.9°   |
| 2ORI   | A     | 44.6°    | 113.0°   |
|        | B     | 44.3°    | 112.2°   |
| 2OSB   | A     | 44.0°    | 113.1°   |
|        | B     | 44.1°    | 112.0°   |
| 2P3S   | A     | 44.2°    | 110.8°   |
| 2RGX   | A     | 44.7°    | 123.2°   |
| 2RH5   | A     | 68.2°    | 141.1°   |
|        | B     | 68.1°    | 139.7°   |
|        | C     | 68.6°    | 141.9°   |
| 3AKY   | A     | 43.7°    | 111.2°   |
| 4AKE   | A     | 74.7°    | 145.9°   |
|        | B     | 74.0°    | 141.7°   |

The NMP-CORE angle and LID-CORE angle for *E. coli* AdK (AK<sub>eco</sub>) or models of AK<sub>eco</sub> based on crystal structures of homologous proteins [1] were computed from the C<sub>α</sub> atoms in the NMP, LID and CORE domain as described in Methods. The structures and structural models are available in the *AKeco Structure Library* under a Creative-Commons Attribution ShareAlike License [2].
