# Supplementary material for: Path Similarity Analysis: a Method for Quantifying Macromolecular Pathways
Source: arXiv:1505.04807 ancillary file (2015-10-23)
Supplement: Supplementary file 7 [file S7_Text.pdf]

# Supporting Information

**S7 Text.** **Discussion of FRODA trajectories as a superset of other trajectory-generating algorithms.**

**In this text we qualitatively discuss the difference between the adenylate kinase (AdK) and diphtheria toxin transition (DT). These differences rationalize the observation that for the DT transition some FRODA trajectories overlap with the ensemble of DIMS trajectories, whereas no such overlap was observed in the case of AdK.**

## Discussion

In the comparison of ensembles of DIMS and FRODA transitions of diphtheria toxin (DT), five FRODA paths were among the cluster of DIMS paths, whereas there was no intermixing between DIMS and FRODA among AdK trajectories. The observation of intermixing supports the idea that the geometrical targeting procedure of FRODA is able to sample the space of trajectories accessible to the force field-based DIMS MD. However, the absence of intermixing in the AdK transitions appears to contradict the idea that FRODA samples a super-space of stereochemically correct transitions. We argue that the absence of overlap between AdK paths generated by FRODA and DIMS is a sampling problem and that—although stereochemically possible—a “DIMS-like” path is nevertheless very rarely sampled by FRODA. In the following, we outline why it is plausible that FRODA does not sample the AdK DIMS transitions.

When both biasing and the potential energy landscape are removed, all of configuration space is in principle uniformly accessible. With rmsd-to-target biasing, paths should coincide with LinInt (as discussed for TMD-F vs LinInt in the main text). Adding stochasticity would generate an ensemble of paths perturbed about LinInt. With the potential landscape and stochasticity (but no biasing), we expect configuration space sampling to be described by equilibrium statistical mechanics. In the case where moderate biasing, a potential landscape, and stochasticity are all present, motion orthogonal to LinInt will be induced by potential barriers and partly by random fluctuations—biasing pulls configurations toward the target so that paths will tend to hug the potential barriers toward LinInt. Now consider a protein with two native states. If no substantial energy barriers exist along the LinInt path, DIMS and FRODA will produce relatively similar pathways (about LinInt) due to the linear nature of their biasing; moreover, if *only* stereochemical barriers are present along LinInt, they should produce paths that wrap around the barriers somewhat closely. If only electrostatic barriers are present along LinInt, DIMS paths will detour around those barriers, while FRODA transitions can proceed uninhibited along LinInt because DIMS—unlike FRODA—takes electrostatics (and other non-bonded interactions) into account.

In AdK angle-angle space, DIMS favors a LID-opening-first pathway, but FRODA samples around LinInt (with LID and NMP opening in tandem). The Hausdorff pairs analysis suggests that several salt bridges impede NMP opening, while the LID opens relatively freely. These electrostatic

interactions are accounted for in DIMS but not in FRODA and are responsible for the difference in DIMS and FRODA paths. DIMS samples conformations with the NMP domain held in place by the salt bridges because the forces directly influence the MD simulation. FRODA, on the other hand, is not driven by forces but relies on rapid sampling of conformation space, and it appears that these very specific salt bridge interactions, which require simultaneous pairings of multiple residues on different domains, belong to unlikely conformations. Therefore, DIMS paths move away from the LinInt path, around the free energy barrier due to the "salt bridge zipper" [1] whereas FRODA follows LinInt and might only rarely sample conformations away from LinInt.

As with AdK, the DT transition can be roughly decomposed into two large-scale motions: the T domain can swing open about the C and R domains as well as rotate about its center of mass. Both DIMS and FRODA generate DT transitions that visually show roughly concurrent opening and rotating of the T domain, although an absence of good known collective variables makes it difficult to accurately describe these motions. Even though DT has salt bridges between the T domain and C/R domains that could alter the coupling of those motions, they appear to interfere with the opening/rotating motions to a lesser degree than in AdK and hence some limited overlap of FRODA trajectories with the DIMS ensemble can be observed.

Although our discussion rationalizes the DIMS/FRODA ensemble comparison clusterings, it would be fruitful to test the hypothesis that electrostatic interactions and the specific form of the progress variable (rmsd in this case) largely shape the overlap between transition path ensembles between DIMS and FRODA. These questions could be addressed by adjusting individual force field terms and/or altering the biasing strength and progress variable, but this was deemed outside of the scope of the current work.git add

## References

[1] Beckstein O, Denning EJ, Perilla JR, Woolf TB. Zipping and Unzipping of Adenylate Kinase: Atomistic Insights into the Ensemble of Open ↔ Closed Transitions. J Mol Biol. 2009 Nov;394(1):160–176.
